# Supplementary material for: Reinforcement Learning from Simulation to Real World Autonomous Driving using Digital Twin
Source: arXiv:2211.14874 source file (2022-11-27)
Supplement: Supplementary file 1 [file velocities.tex]

%\begin{figure*}[!t]
%	\centering
%   \subfloat[]{\includegraphics[width=0.33\textwidth]{tikz/velocity0.tikz}%
%		\label{fig:velocity0}}
%	\hfil
%	\subfloat[]{\includegraphics[width=0.33\textwidth]{tikz/velocity1.tikz}%
%		\label{fig:velocity1}}
%    \hfil
%	\subfloat[]{\includegraphics[width=0.33\textwidth]{tikz/velocity2.tikz}%
%		\label{fig:velocity2}}
%    \hfil
%	\subfloat[]{\includegraphics[width=0.33\textwidth]{tikz/velocity3.tikz}%
%		\label{fig:velocity3}}
%    \hfil
%    \subfloat[]{\includegraphics[width=0.33\textwidth]{tikz/velocity4.tikz}%
%		\label{fig:velocity4}}
%	\hfil
%	\subfloat[]{\includegraphics[width=0.33\textwidth]{tikz/velocity5.tikz}%
%		\label{fig:velocity5}}
%    \hfil
%	\subfloat[]{\includegraphics[width=0.33\textwidth]{tikz/velocity6.tikz}%
%		\label{fig:velocity6}}
%    \hfil
%    \subfloat[]{\includegraphics[width=0.33\textwidth]{tikz/velocity7.tikz}%
%		\label{fig:velocity7}}
%	\hfil
%	\subfloat[]{\includegraphics[width=0.33\textwidth]{tikz/velocity8.tikz}%
%		\label{fig:velocity8}}
%   \hfil
%	\subfloat[]{\includegraphics[width=0.33\textwidth]{tikz/velocity9.tikz}%
%		\label{fig:velocity9}}
%    \hfil
%	\caption{Different traffic scenarios for training the path-tracking controller. The data is recorded in the parking lot belonging to Siemens Digital Industries Software in Belgium. The white and blue circles indicate the starting and end positions of the vehicle.}
%	\label{fig:velocity_rw_data}
%\end{figure*}
