# Supplementary material for: Reinforcement Learning from Simulation to Real World Autonomous Driving using Digital Twin
Source: arXiv:2211.14874 source file (2022-11-27)
Supplement: Supplementary file 3 [file implementation.tex]

\begin{figure}
    \centering
    \includegraphics[width=\linewidth]{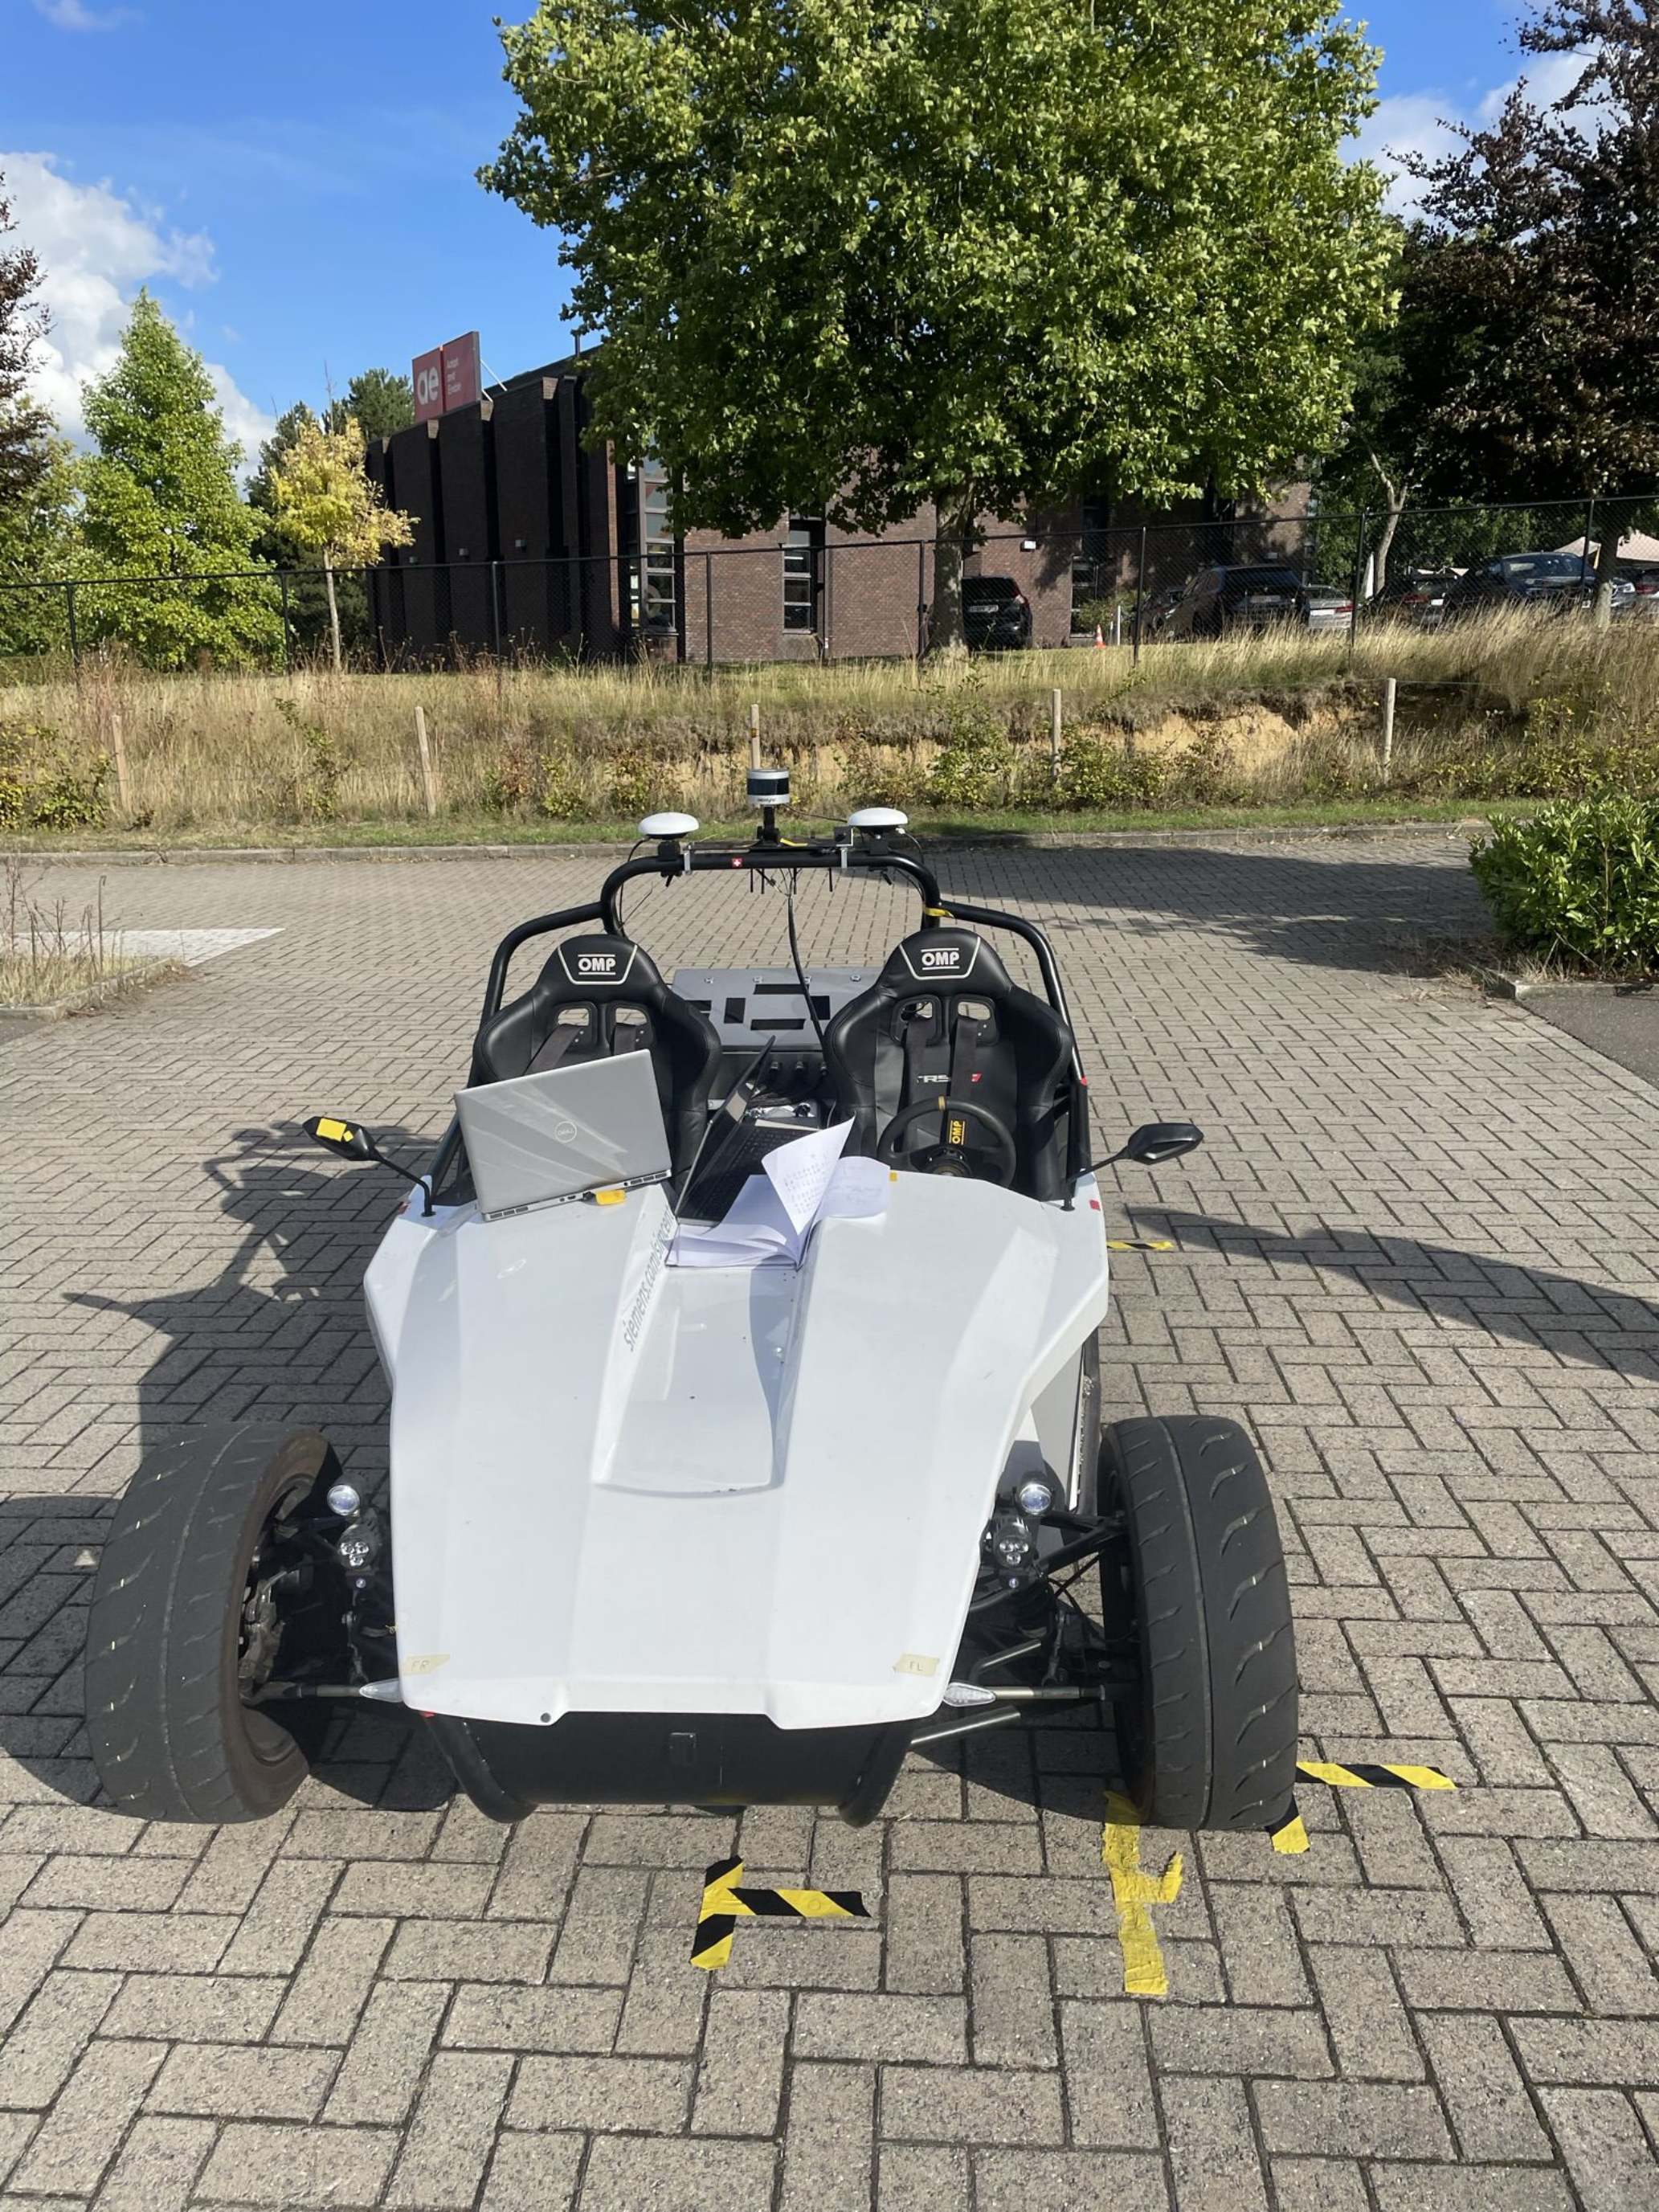}
    \caption{SimRod: the vehicle used for testing with Hehicle-in-the-Loop and Vehicle-in-the-Loop. The PC connected is used to visualize the states fed to the actor and log data to compare afterwards.}
    \label{fig:simrod}
\end{figure}
