# Supplementary material for: Reinforcement Learning from Simulation to Real World Autonomous Driving using Digital Twin
Source: arXiv:2211.14874 source file (2022-11-27)
Supplement: Supplementary file 6 [file rw_mil.tex]

\begin{figure*}[tb]
	\centering
        \subfloat[]{\includegraphics[width=0.3\textwidth]{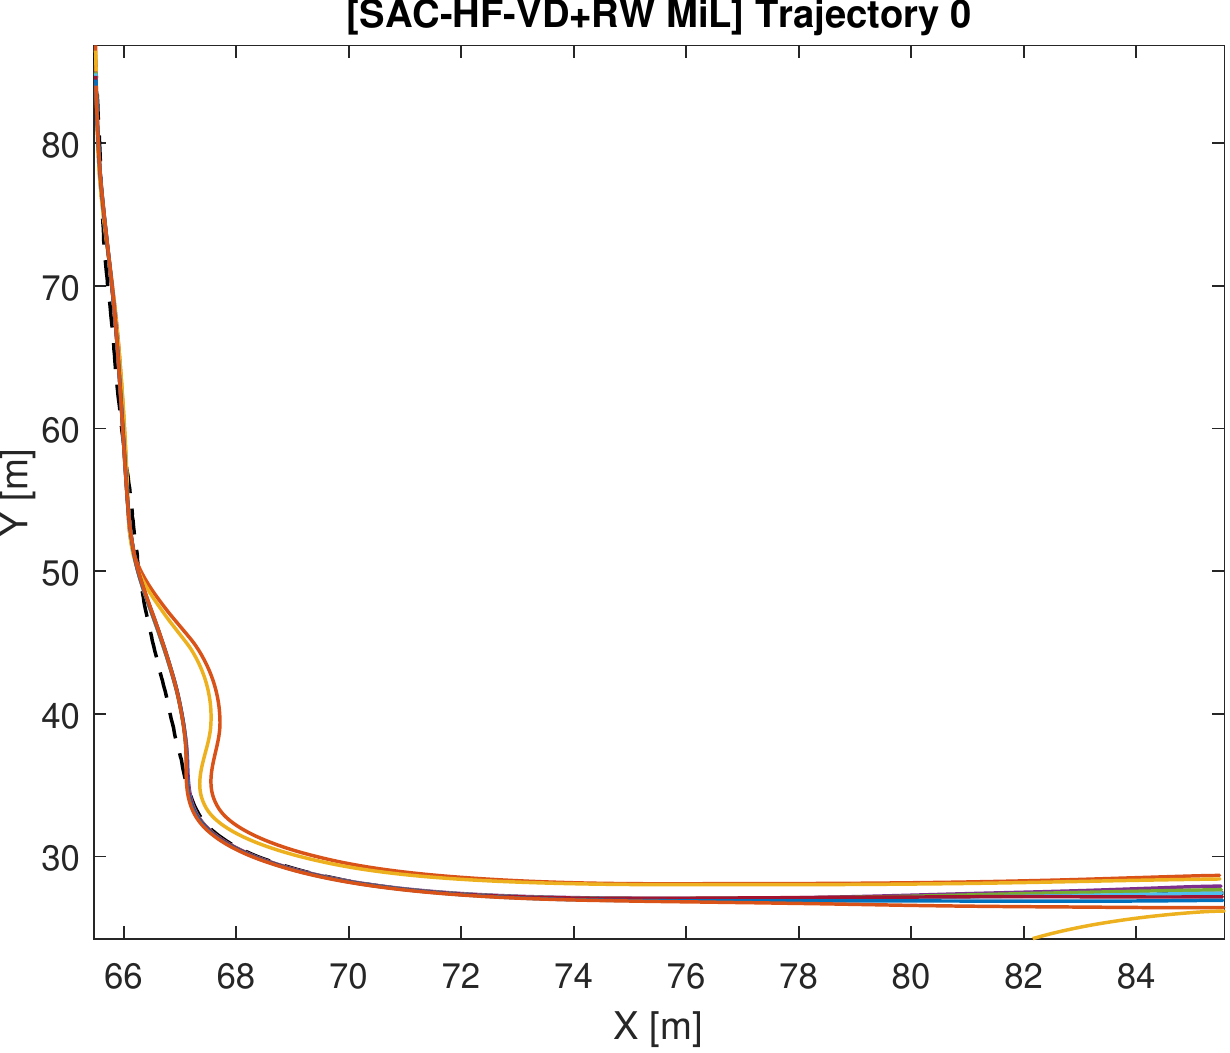}%
		\label{fig:rw_mil_traj0}}
    \hfil
	\subfloat[]{\includegraphics[width=0.3\textwidth]{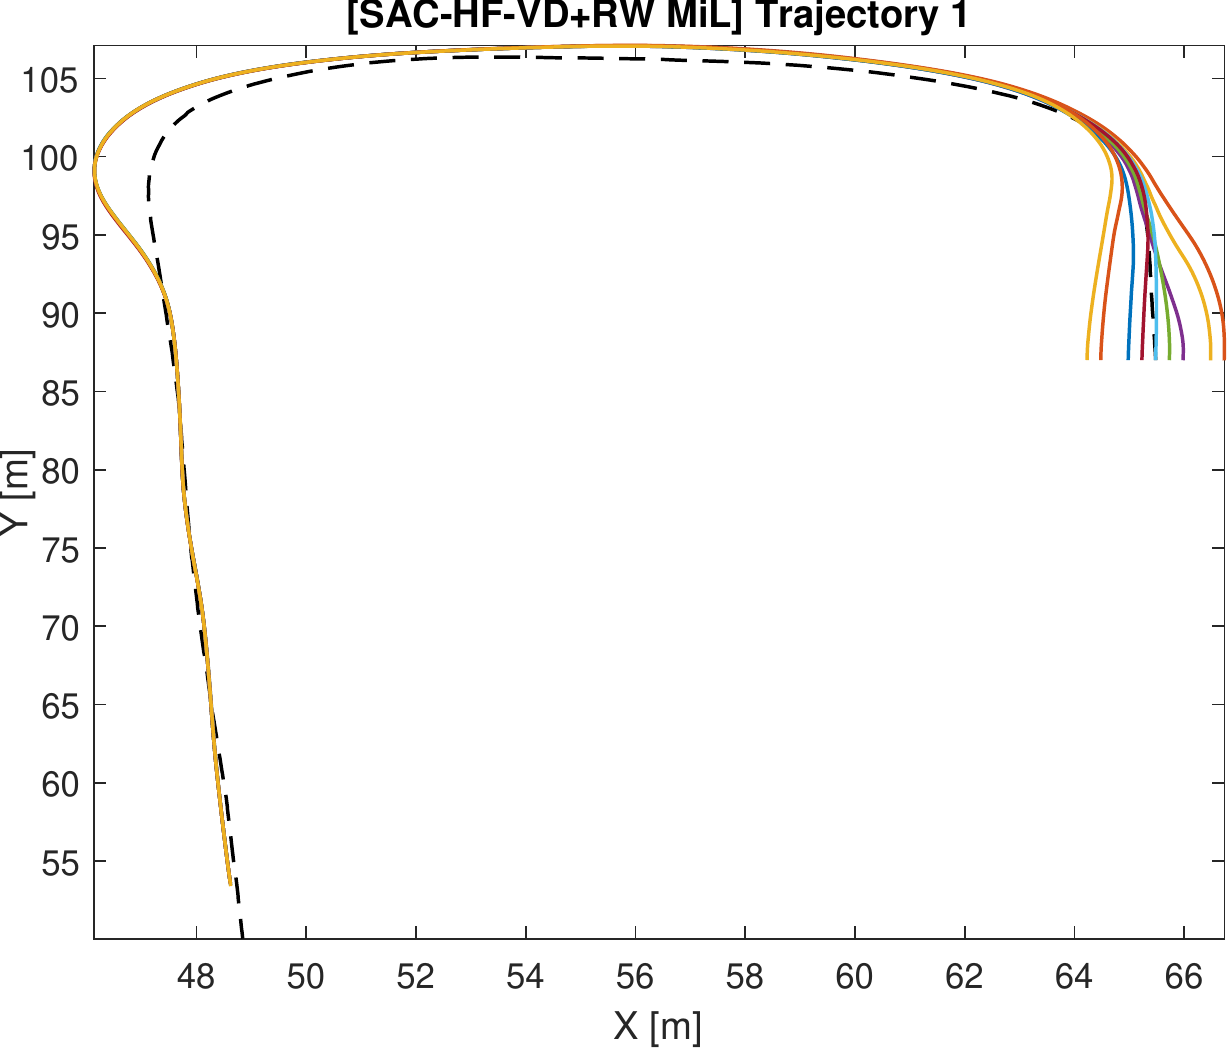}%
		\label{fig:rw_mil_traj1}}
    \hfil
	\subfloat[]{\includegraphics[width=0.3\textwidth]{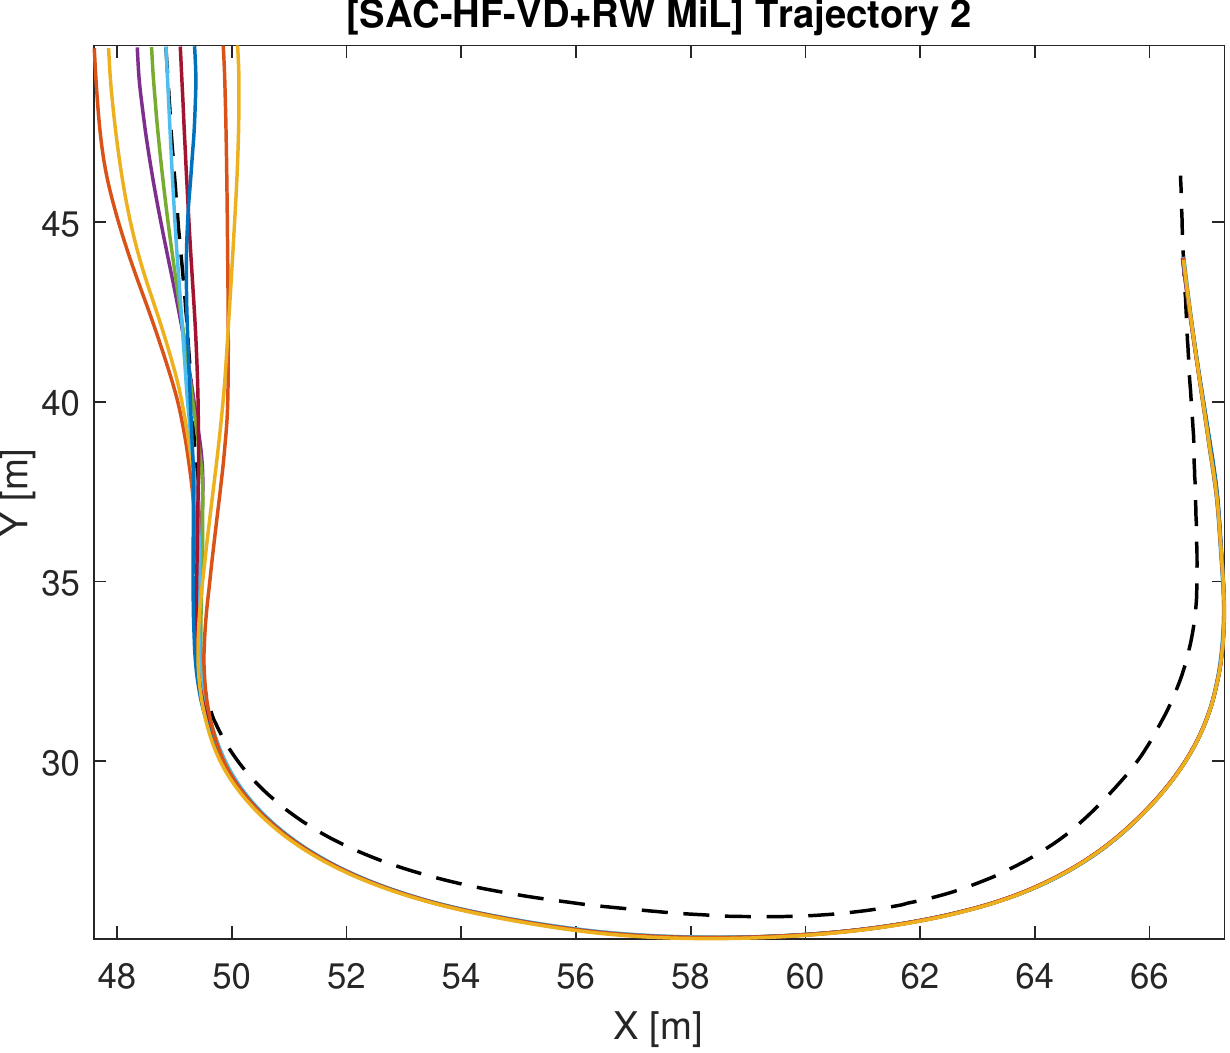}%
		\label{fig:rw_mil_traj2}}
    \hfil
	\subfloat[]{\includegraphics[width=0.3\textwidth]{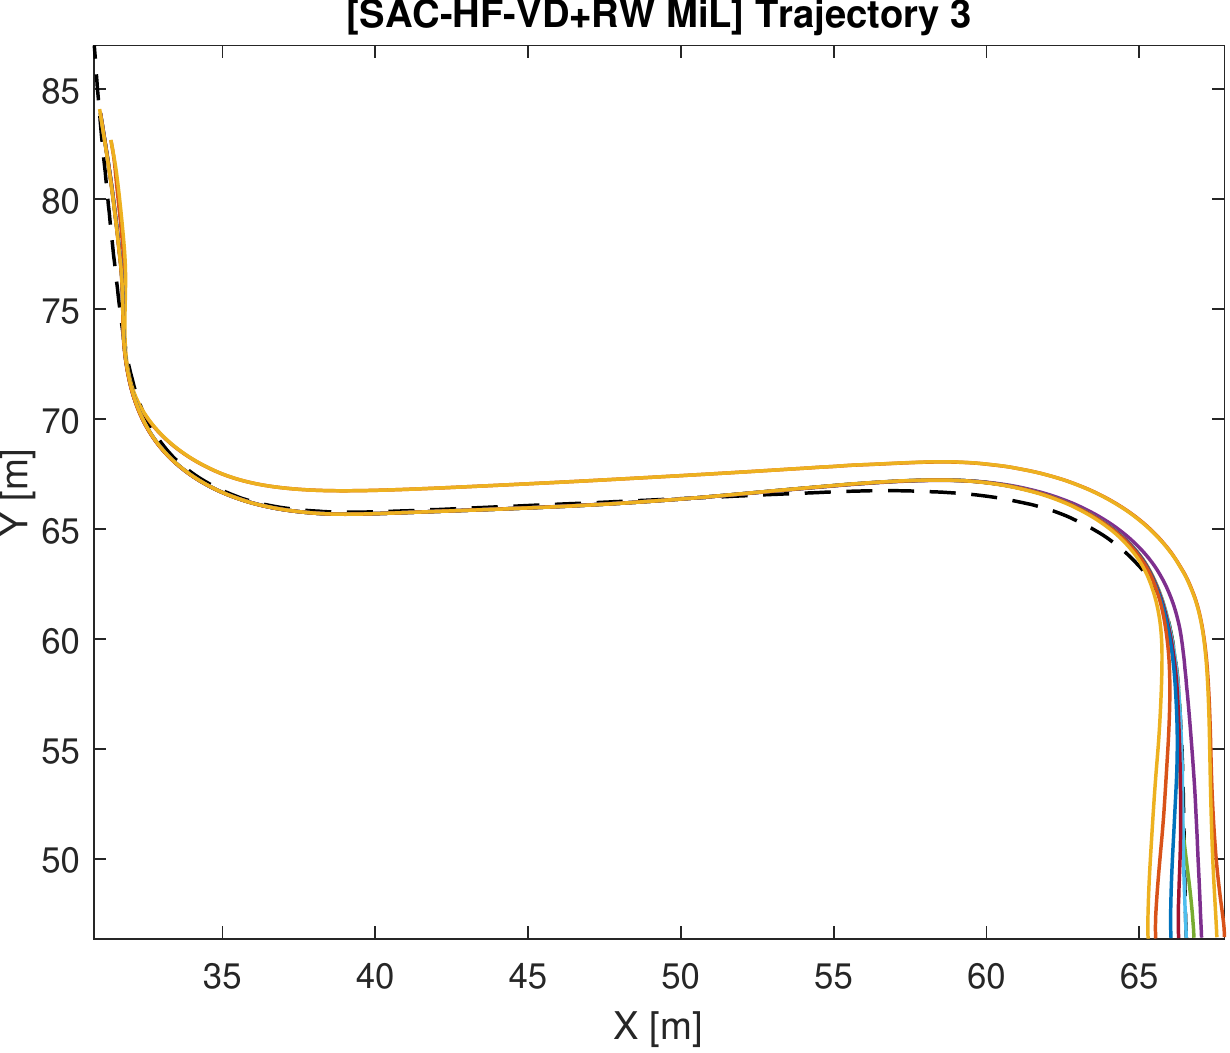}%
		\label{fig:rw_mil_traj3}}
    \hfil
        \subfloat[]{\includegraphics[width=0.3\textwidth]{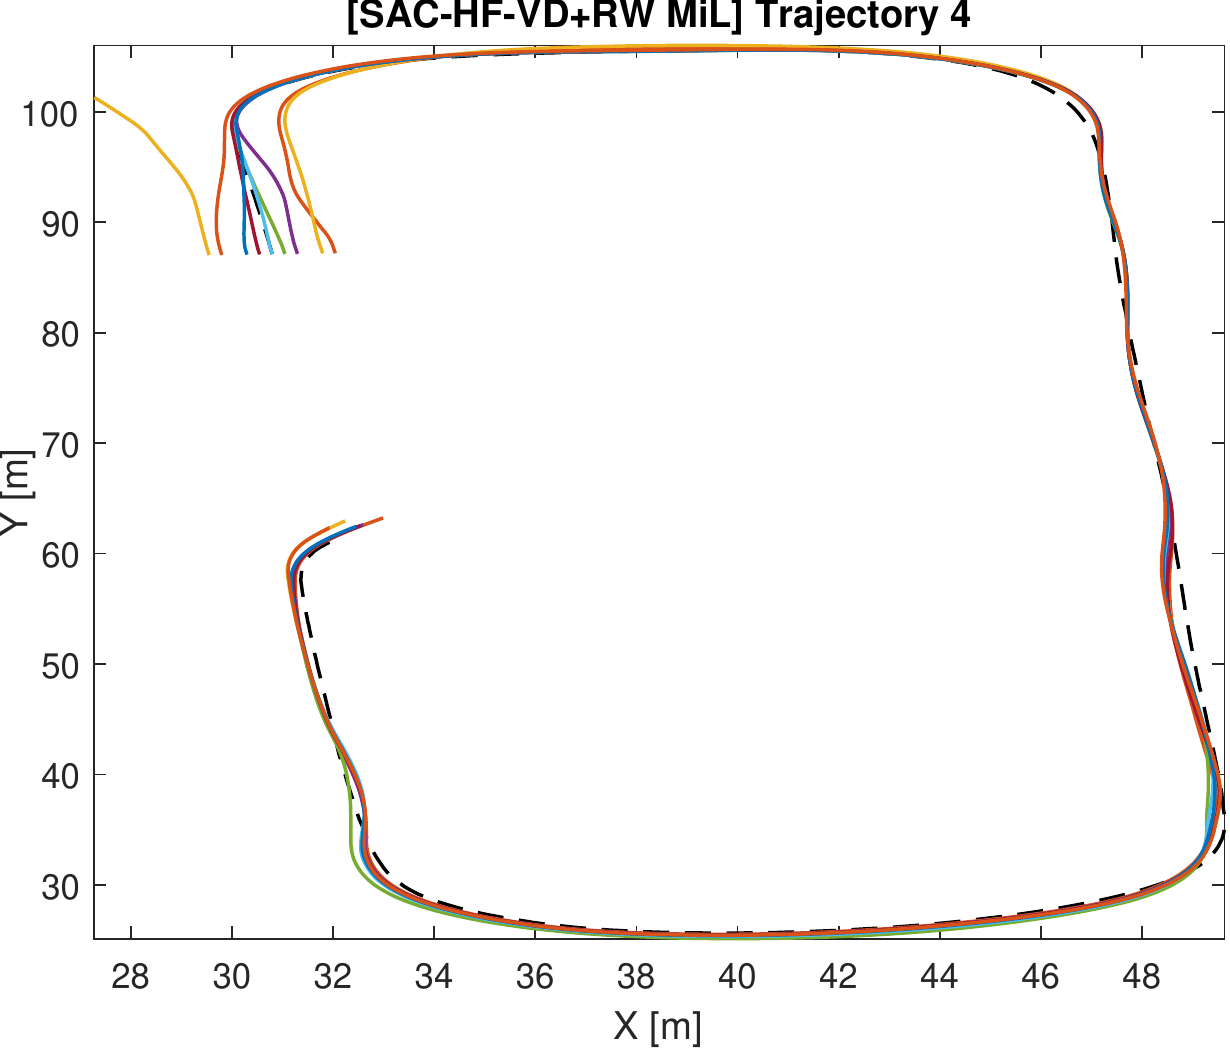}%
		\label{fig:rw_mil_traj4}}
    \hfil
	\subfloat[]{\includegraphics[width=0.3\textwidth]{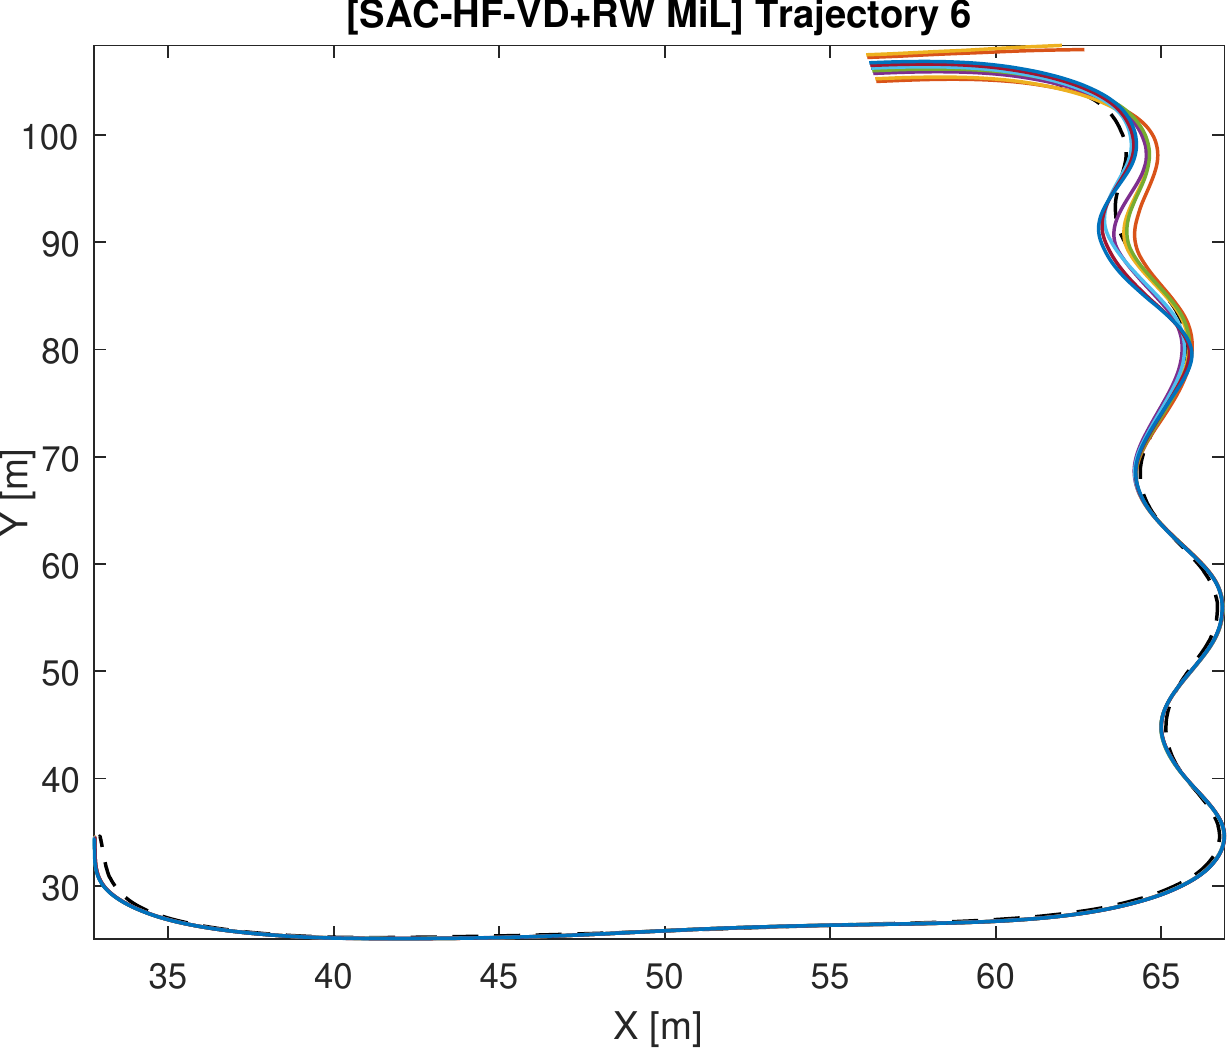}%
		\label{fig:rw_mil_traj6}}
    \hfil
	\subfloat[]{\includegraphics[width=0.3\textwidth]{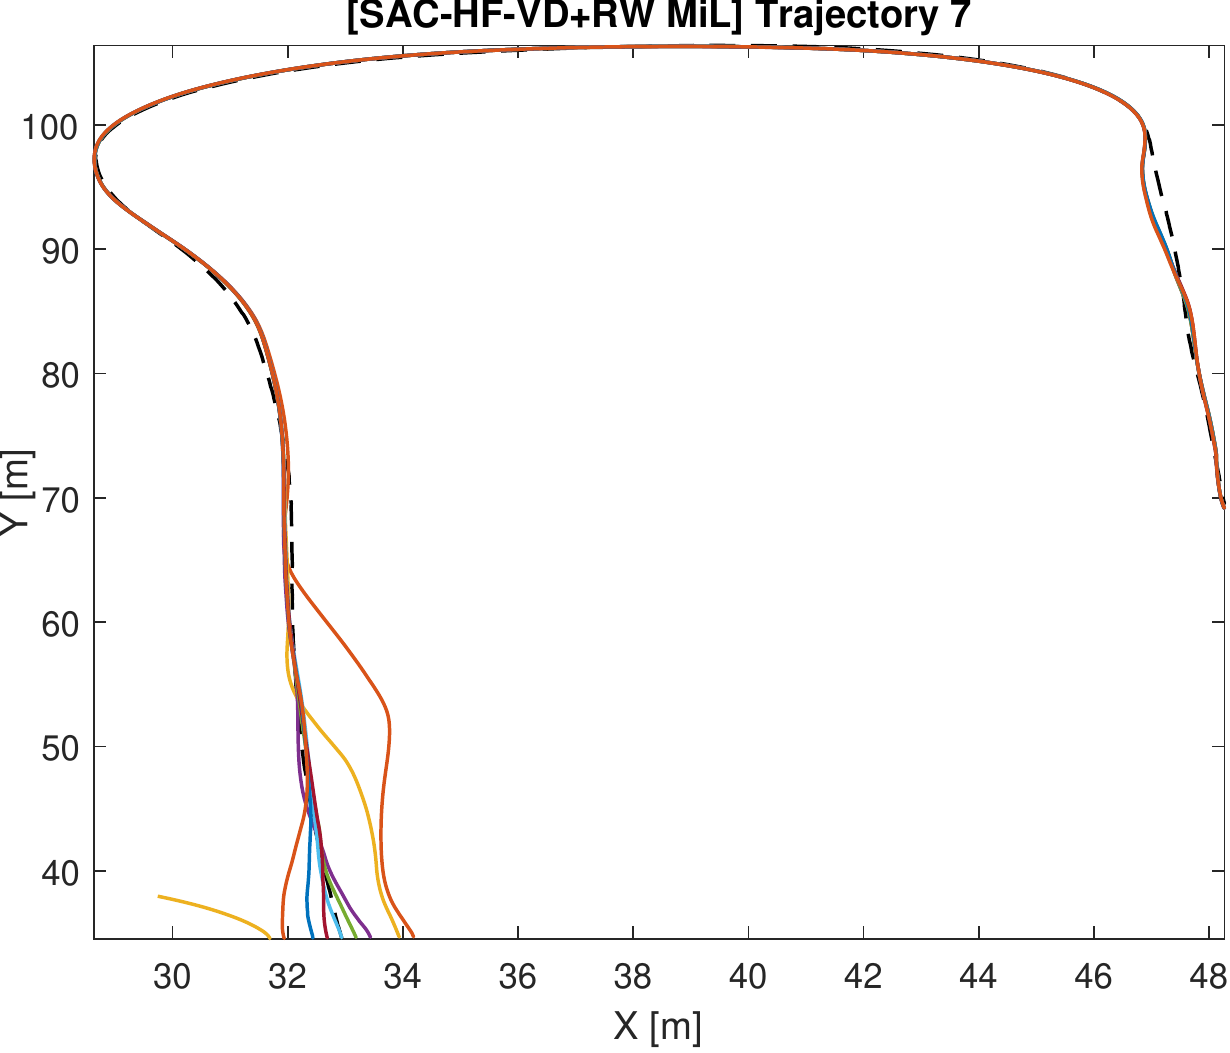}%
		\label{fig:rw_mil_traj7}}
    \hfil
        \subfloat[]{\includegraphics[width=0.3\textwidth]{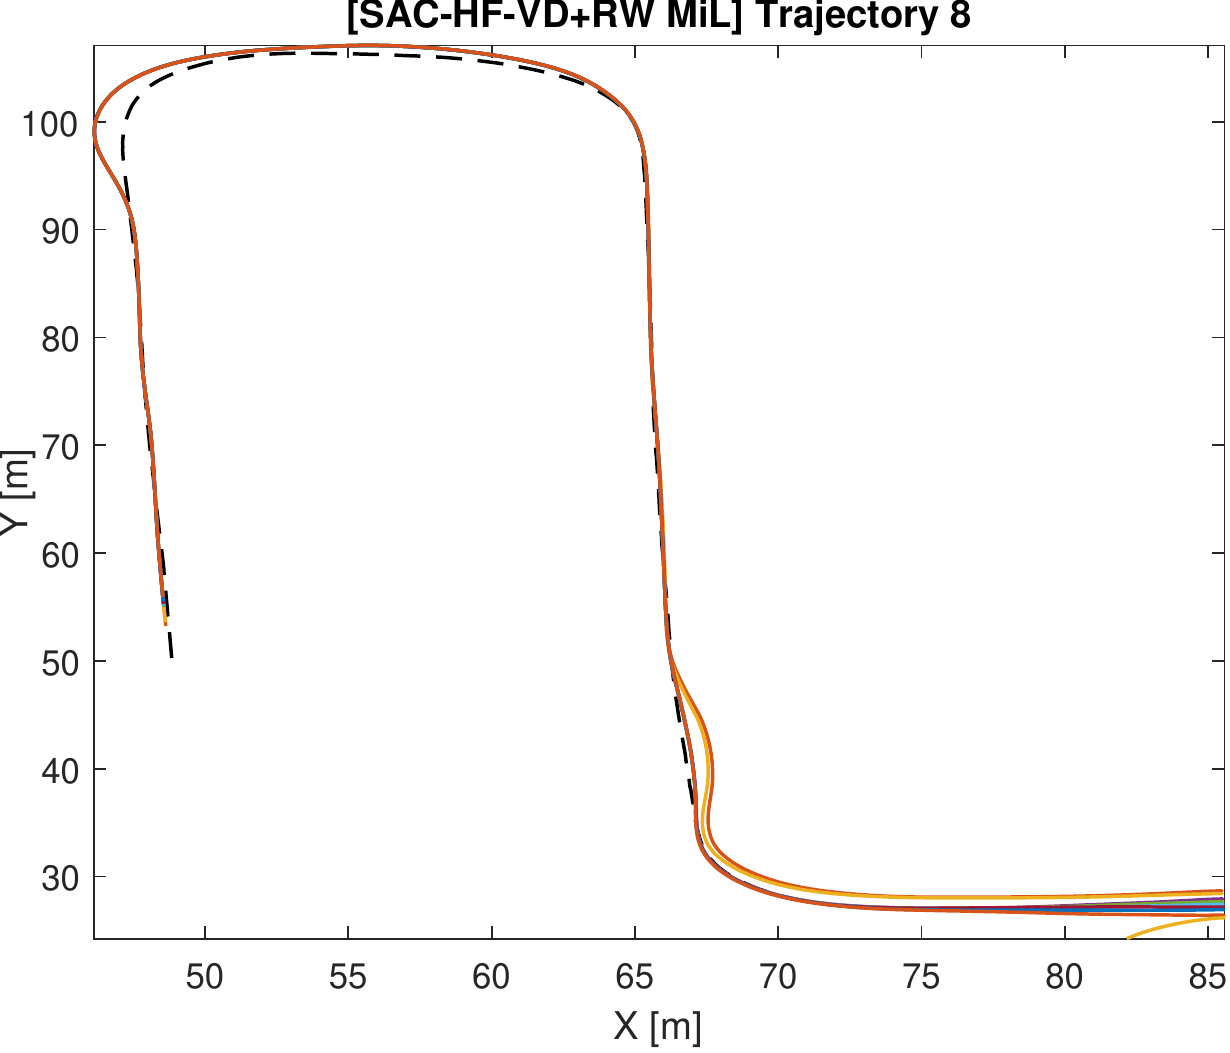}%
		\label{fig:rw_mil_traj8}}
      \hfil
        \subfloat[]{\includegraphics[width=0.3\textwidth]{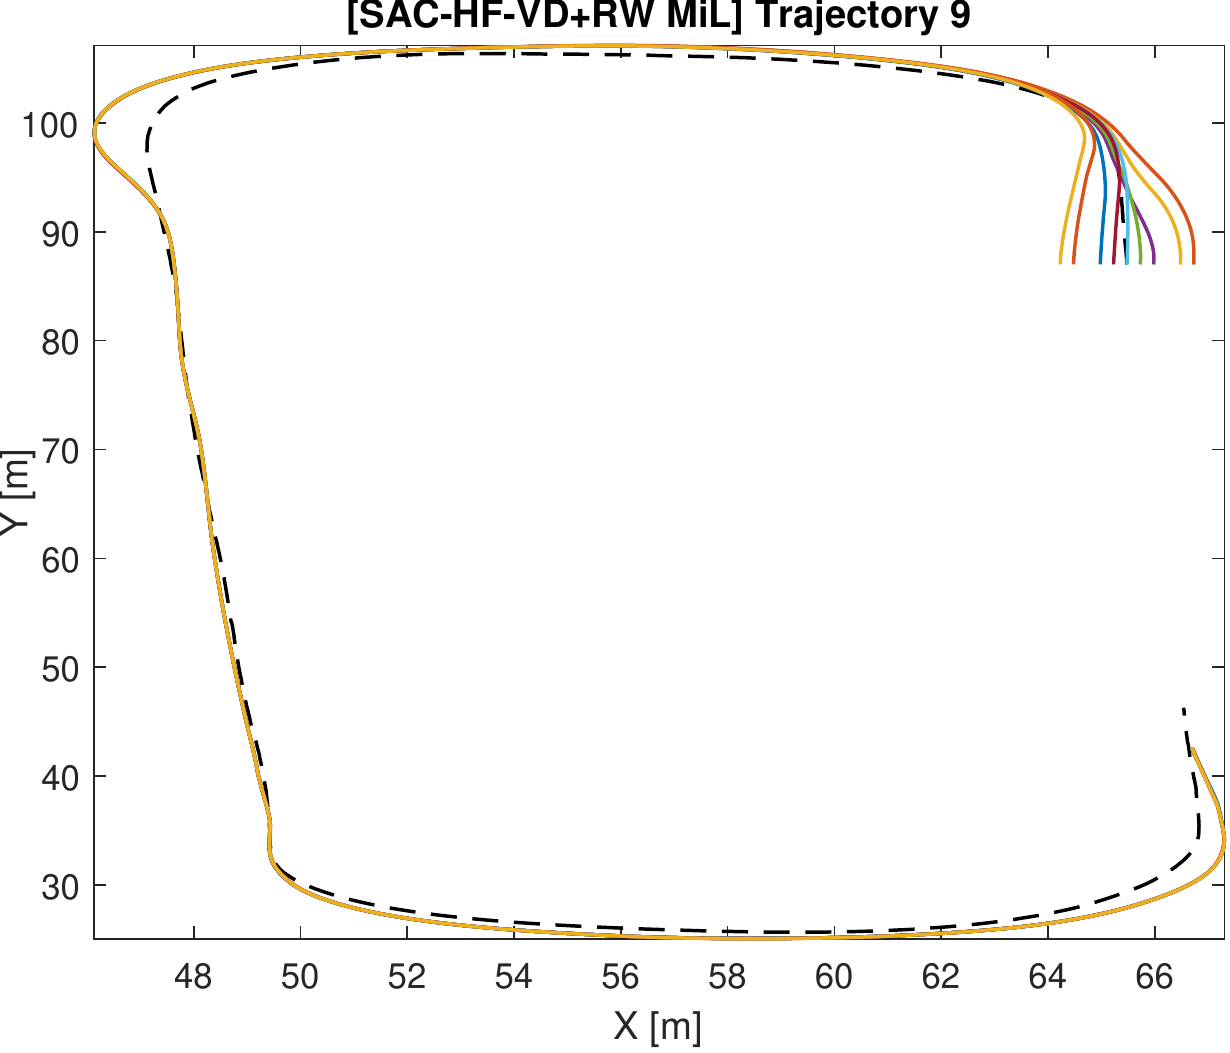}%
		\label{fig:rw_mil_traj9}}
    \caption{Model-in-the-loop results for the SAC agent trained with the high-fidelity (HF) model and finetuned with real-world data (RW) and tested with different initial lateral deviations.}
    \label{fig:rw_mil}
\end{figure*}
