# Supplementary material for: Reinforcement Learning from Simulation to Real World Autonomous Driving using Digital Twin
Source: arXiv:2211.14874 source file (2022-11-27)
Supplement: Supplementary file 9 [file vil_4.tex]

\begin{figure*}[tb]
    \centering
        \subfloat[]{\includegraphics[width=0.33\textwidth]{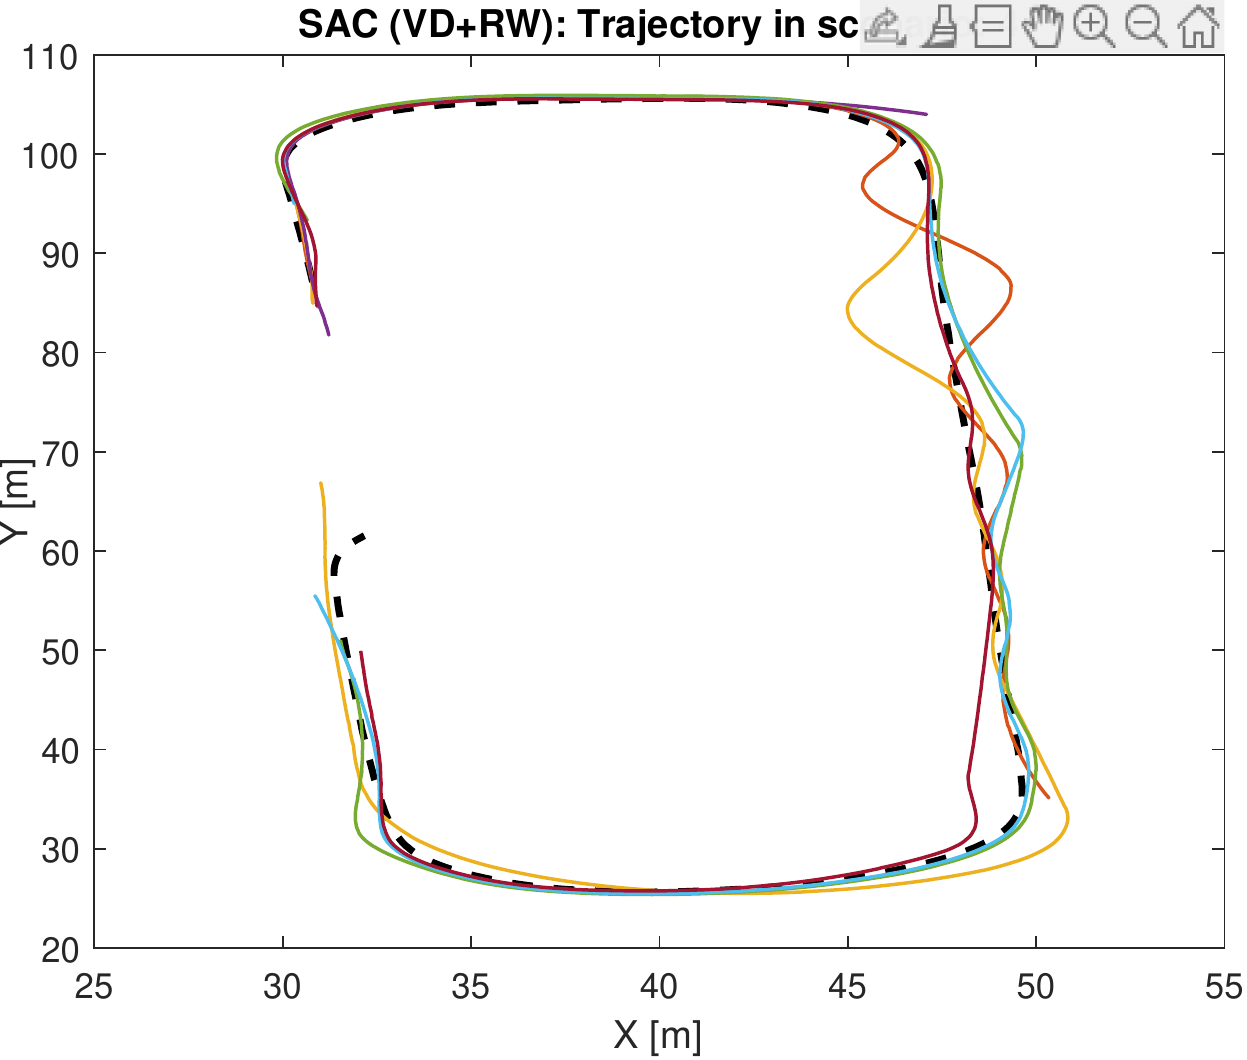}%
		\label{fig:rw_vil_traj4}}
    \hfil
        \subfloat[]{\includegraphics[width=0.33\textwidth]{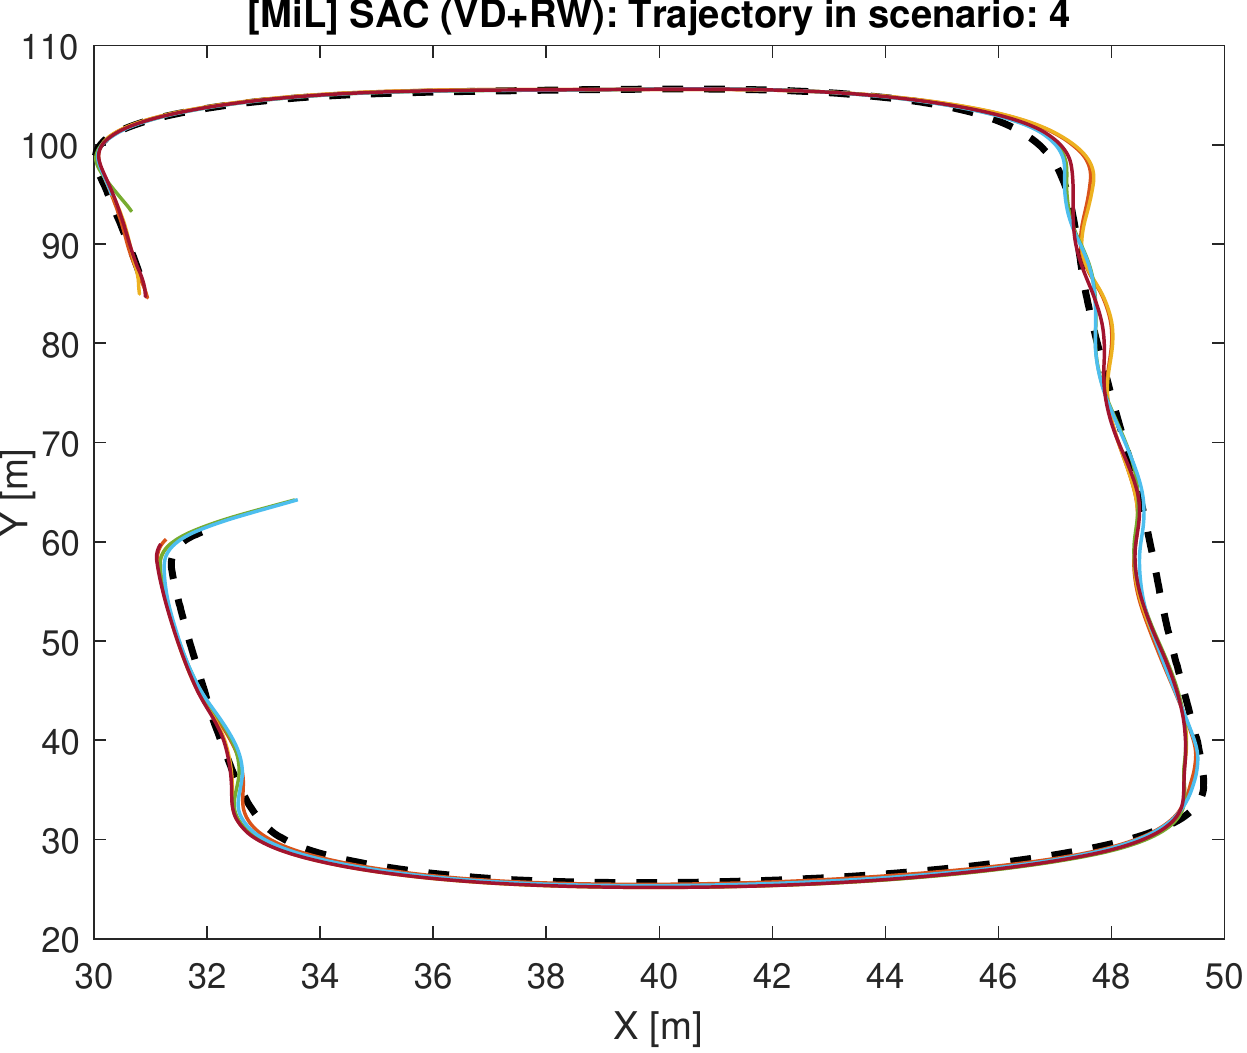}%
		\label{fig:rw_vilmil_traj4}}
    \caption{Vehicle in the loop results for scenario 9 and model-in-the-loop results for the SAC-HF-RW agent.}
    \label{fig:vil_traj4}
\end{figure*}
