# Supplementary material for: Reinforcement Learning from Simulation to Real World Autonomous Driving using Digital Twin
Source: arXiv:2211.14874 source file (2022-11-27)
Supplement: Supplementary file 10 [file vil_6.tex]

\begin{figure*}[tb]
    \centering
        \subfloat[]{\includegraphics[width=0.33\textwidth]{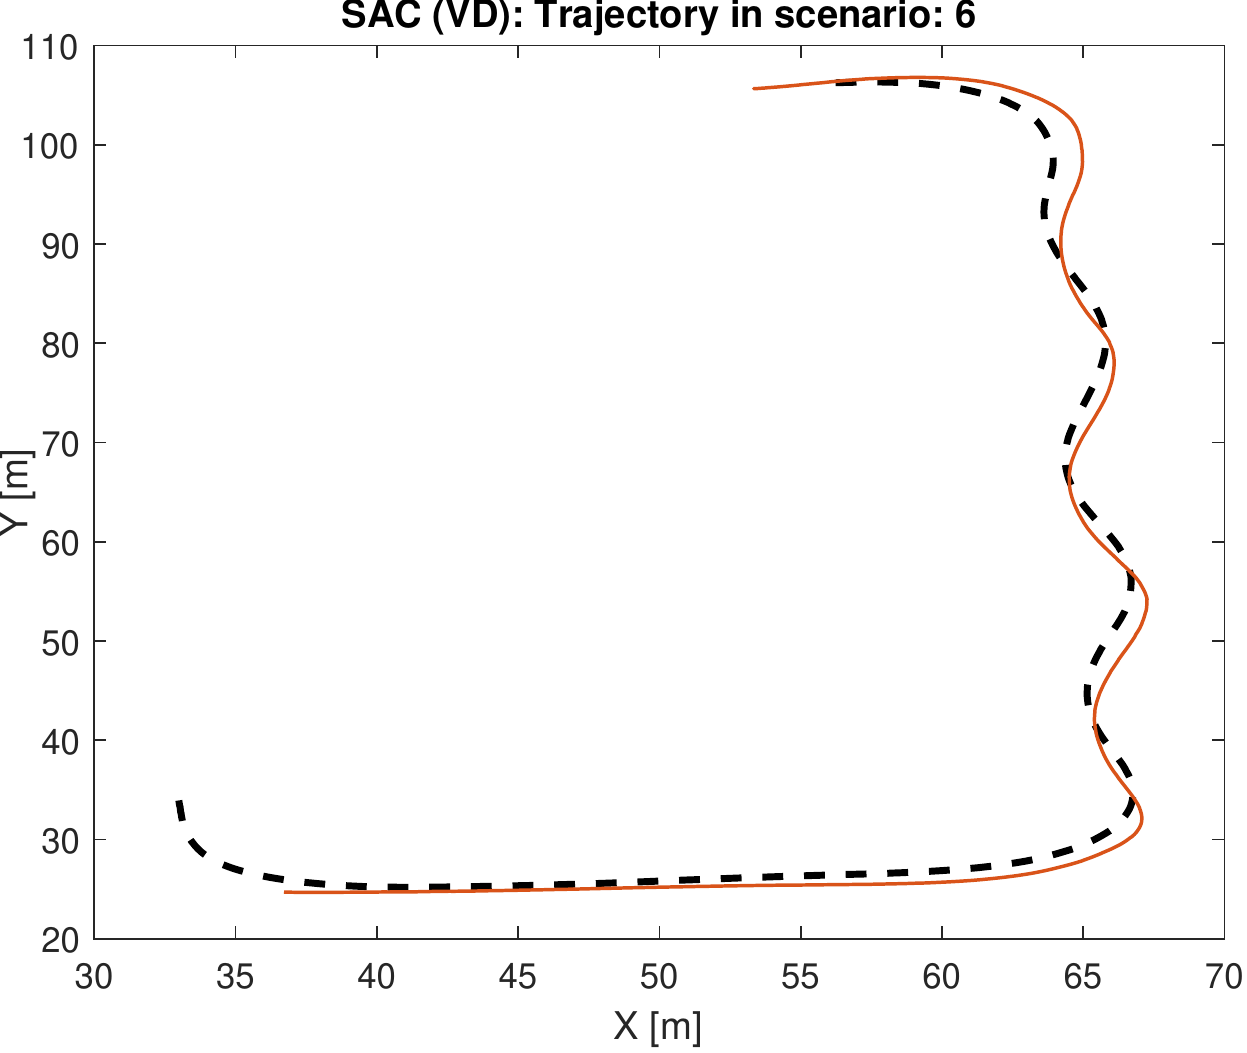}%
            \label{fig:ps_vil_traj6}}
    \hfil
        \subfloat[]{\includegraphics[width=0.33\textwidth]{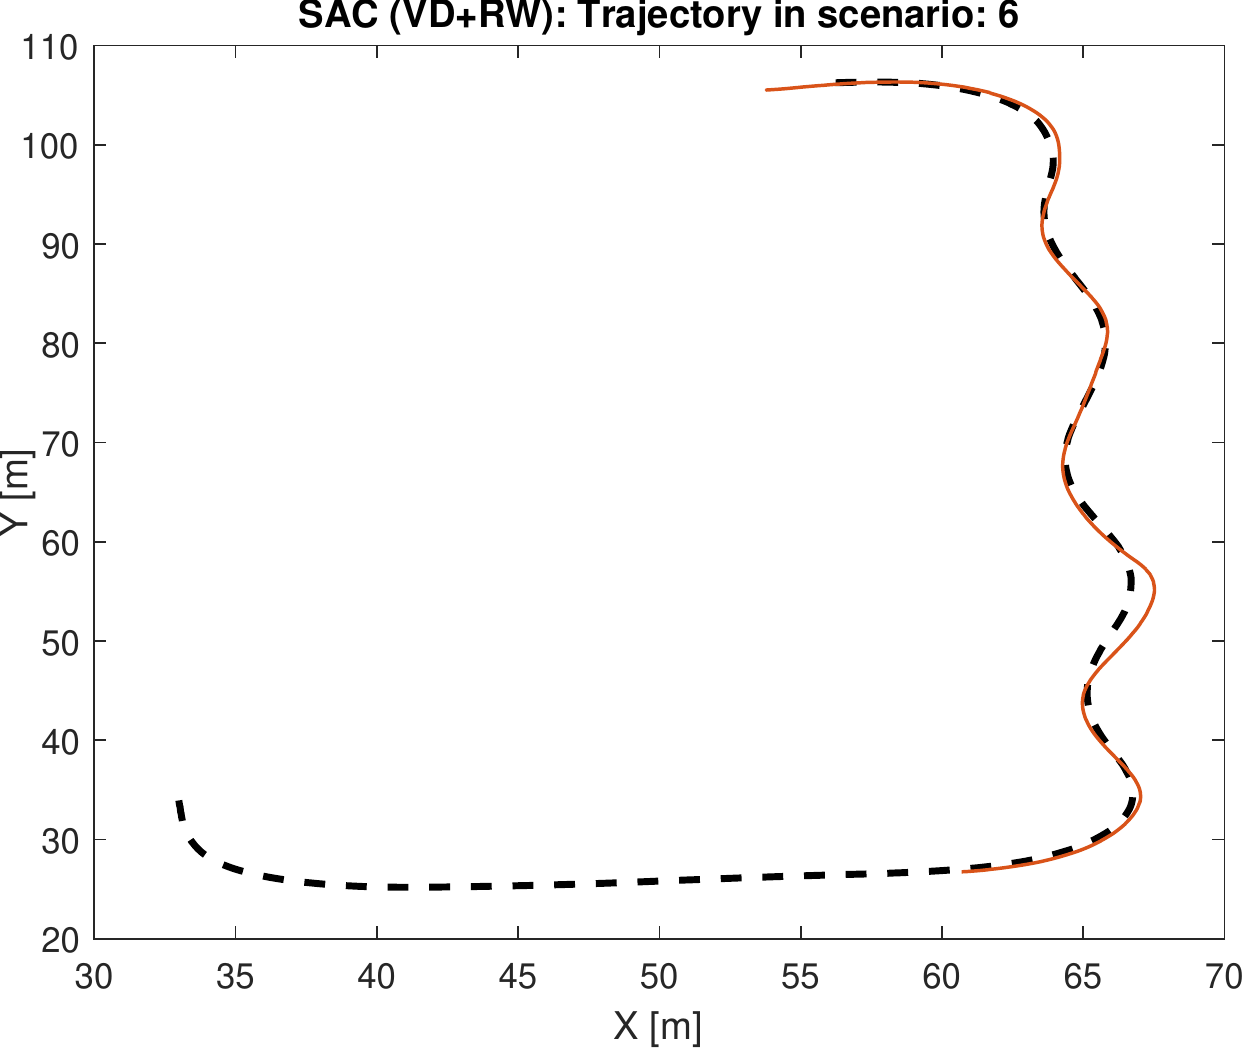}%
		\label{fig:rw_vil_traj6}}
    \hfil
	\subfloat[]{\includegraphics[width=0.33\textwidth]{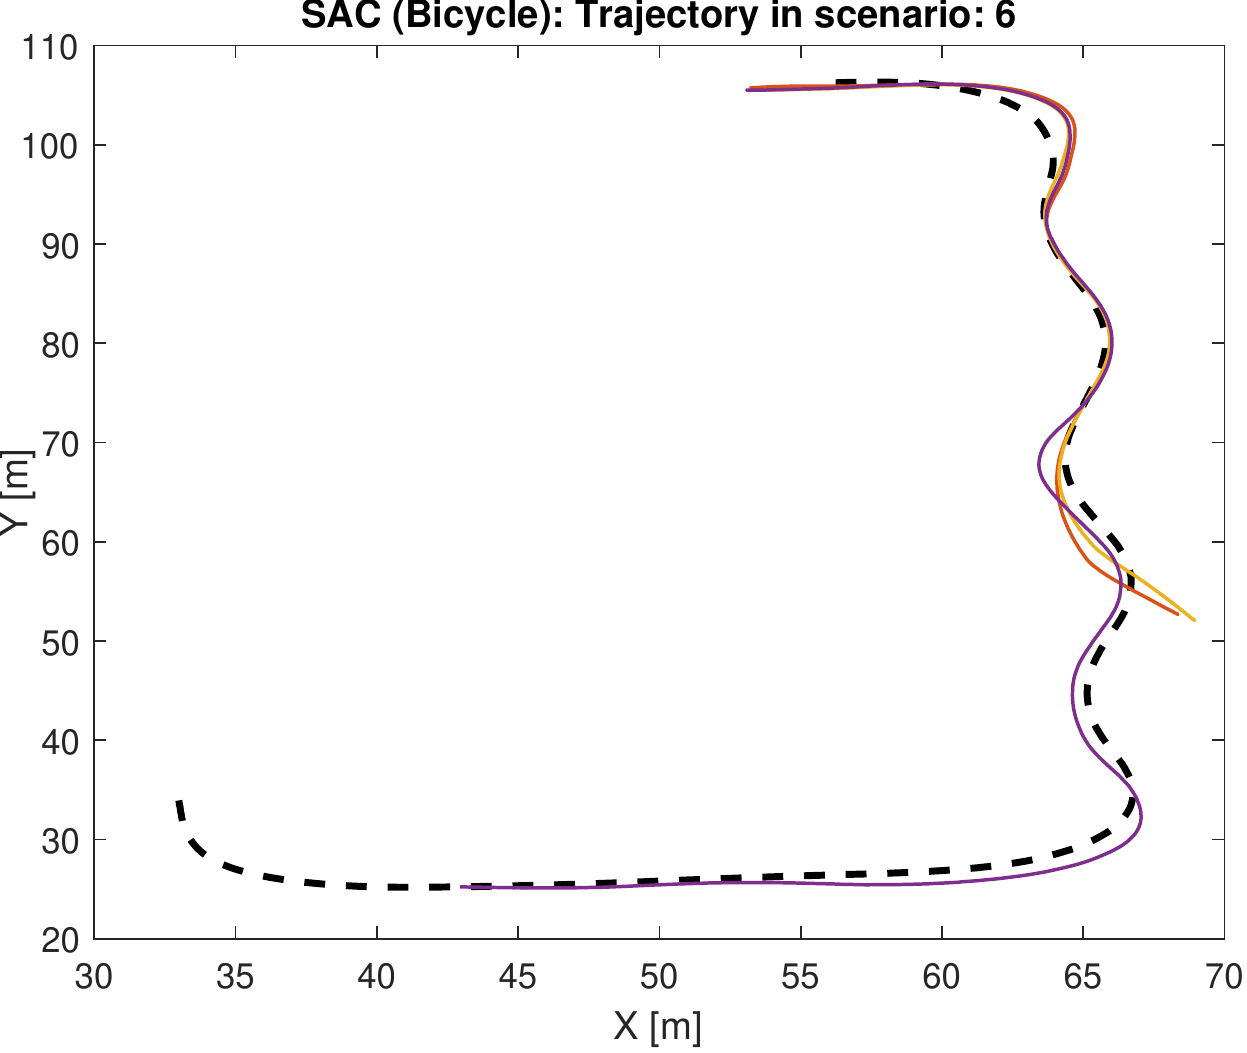}%
		\label{fig:bicycle_vil_traj6}}
    \hfil
        \subfloat[]{\includegraphics[width=0.33\textwidth]{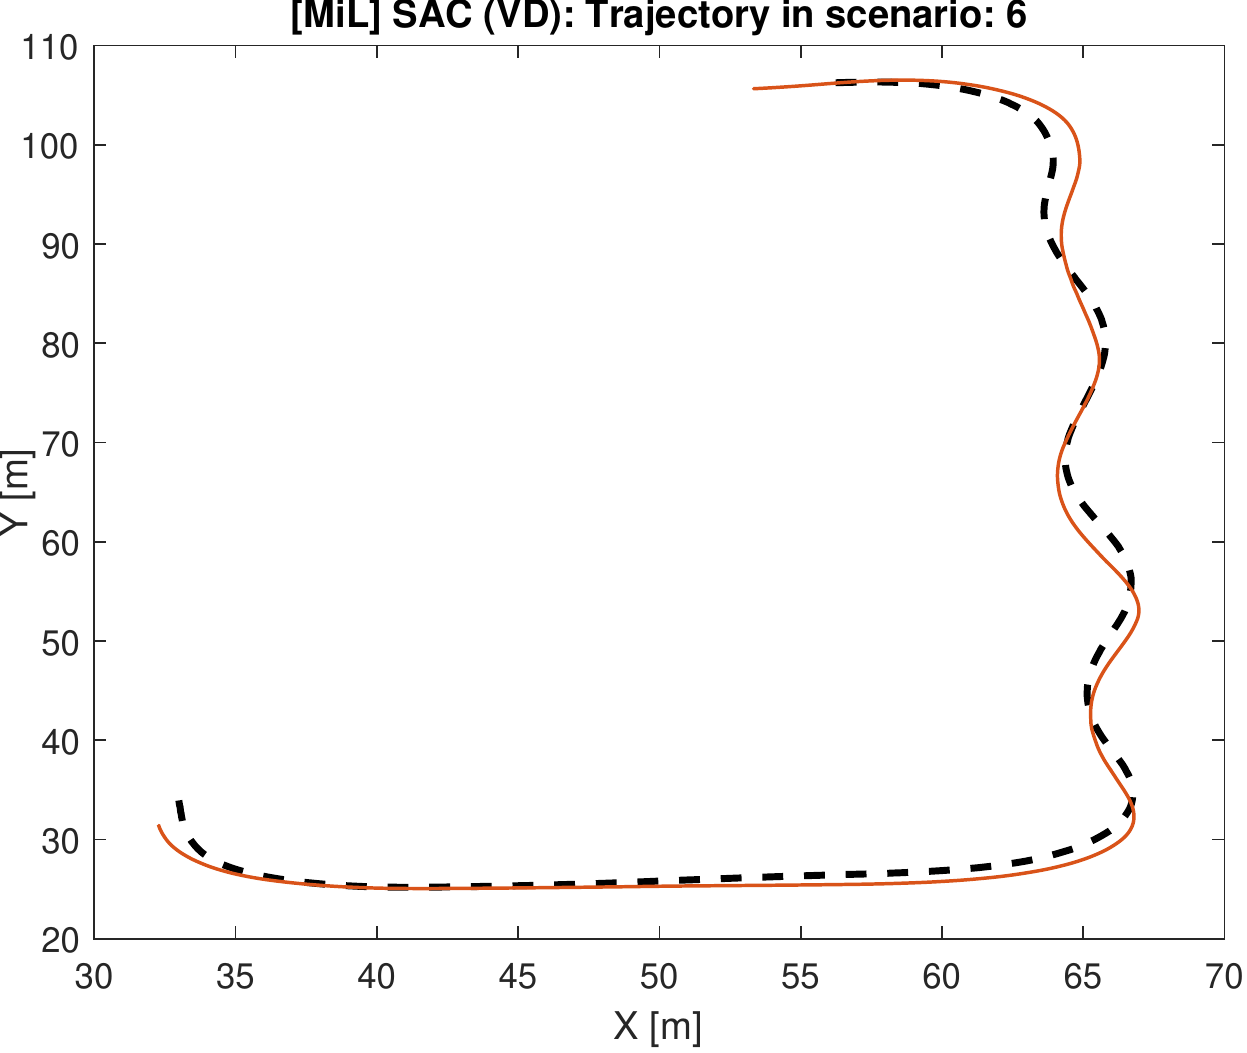}%
            \label{fig:ps_vilmil_traj6}}
    \hfil
        \subfloat[]{\includegraphics[width=0.33\textwidth]{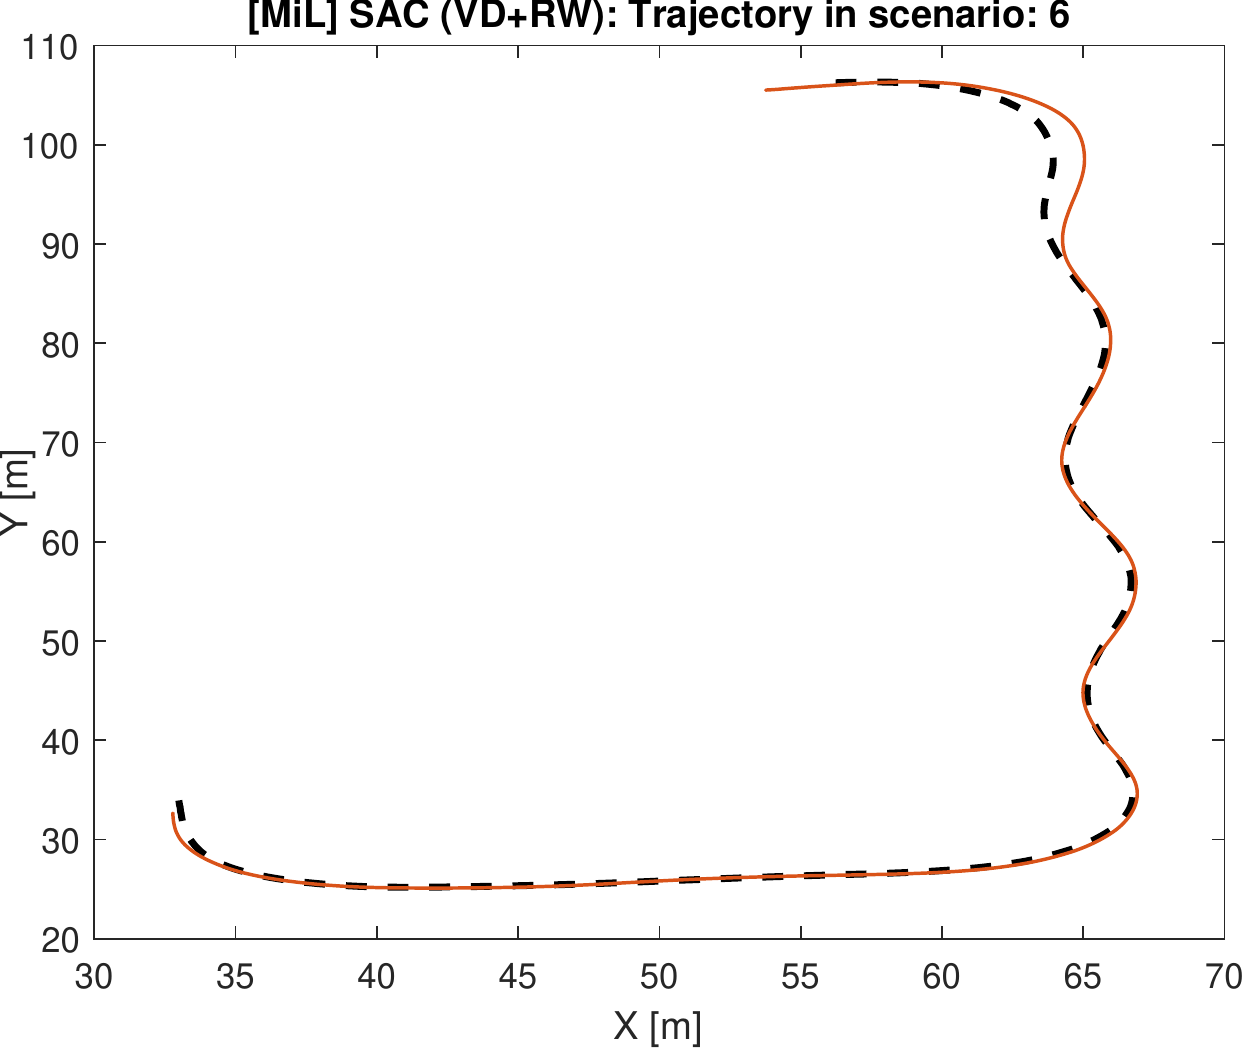}%
		\label{fig:rw_vilmil_traj6}}
    \hfil
	\subfloat[]{\includegraphics[width=0.33\textwidth]{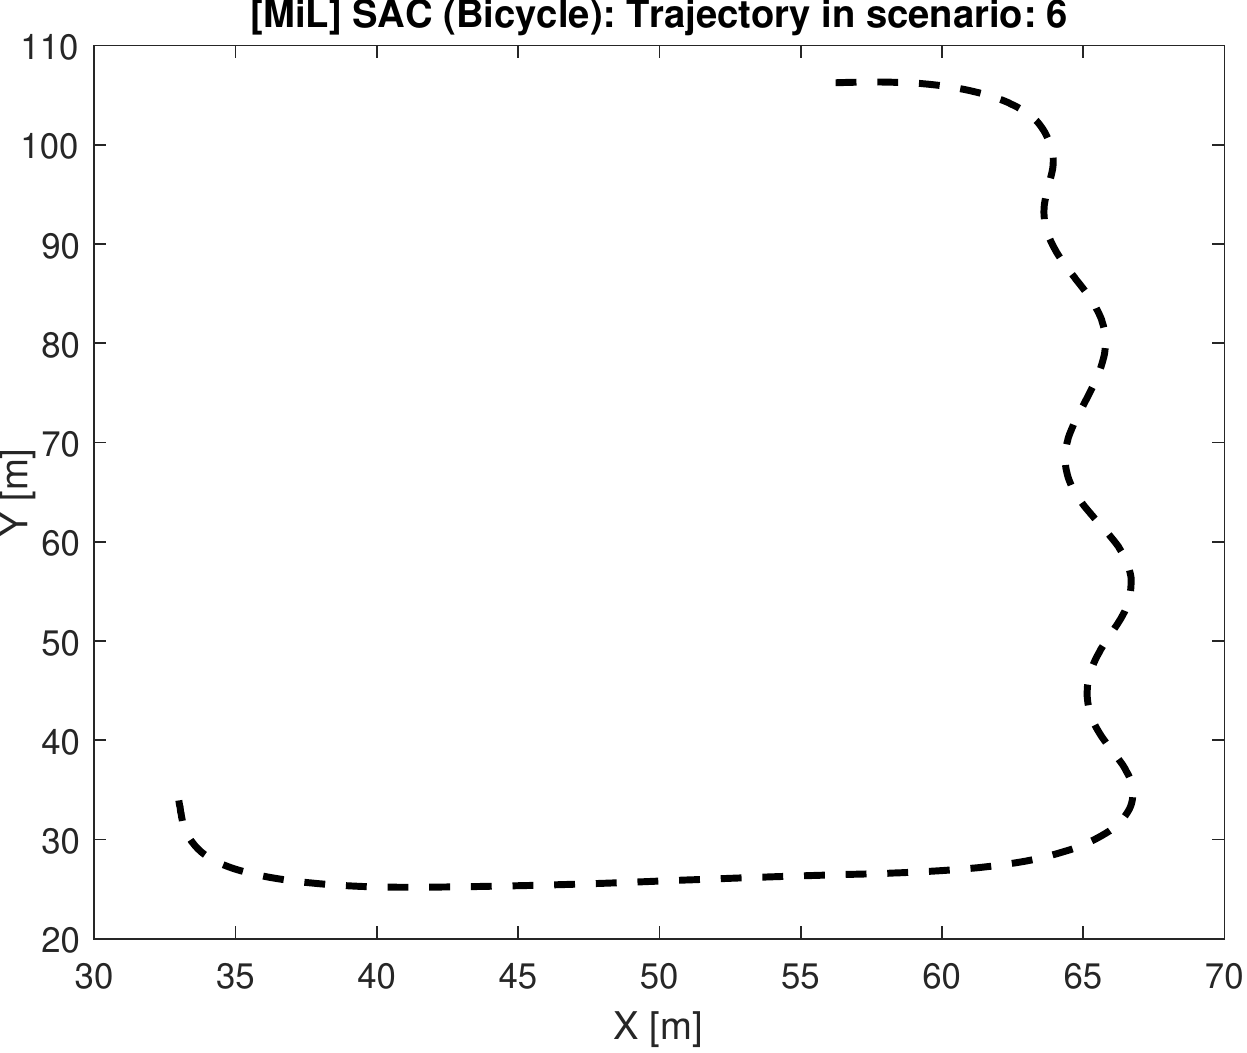}%
		\label{fig:bicycle_vilmil_traj6}}
    \caption{Vehicle in the loop results for scenario 6 (first row) and model-in-the-loop results for the same initial conditions. No MiL results available for the agent trained with the bicycle model.}
    \label{fig:vil_traj6}
\end{figure*}
